# Supplementary material for: Online learning with kernel losses
Source: arXiv:1802.09732 source file (2018-02-27)
Supplement: Supplementary file 2 [file quadraticscovarianceappendix.tex]

Consider the function $f(x) = x^T A x + b^T x $ for a symmetric matrix $A \in \mathbb{R}^{n \times n}$ and vector $b \in \mathbb{R}^n$. 

Let $\Phi(x) = \begin{bmatrix} x(1)^2 \\ . \\ x(n)^2 \\ 2x(1)x(2) \\. \\ 2x({n-1})x(n) \\ x(1) \\. \\x(n) \end{bmatrix}$ 

And abusing notation $\Phi(A,b) = \begin{bmatrix} A_{1,1} \\ . \\ A_{n,n} \\ 2A_{1,2} \\ . \\ 2A_{n-1, n} \\ b_1 \\ . \\ b_n\end{bmatrix}$

Notice that $f(x) = \langle \Phi(x), \Phi(A,b) \rangle$.
